# Supplementary material for: S$^3$R: Fast and Faithful RL Rollouts via Self-Sparse Speculative Decoding
Source: arXiv:2610.13202 source file (2026-11-03)
Supplement: Supplementary file 1 [file sparse_self_speculation_measurements.tex]

% Integrated from figs/why_ssrl_2. Reported numerical results are unchanged.
% Input within Appendix app:why-ssrl, after its component analysis and profiles.

\subsection{Controlled budget--acceptance trade-off}
\label{app:why-ssrl-budget}

We vary the sparse budget while measuring both acceptance and throughput
to test the trade-off in Section~\ref{sec:efficiency-runtime}.
These measurements use real mathematical continuations and complete
GPU-work windows, complementing the component profiles above.

\paragraph{Models and inputs.}
Qwen3-1.7B and Qwen3-8B each use their frozen DAPO step-60 checkpoint,
BF16, two H100 80GB GPUs, TP$=2$, $k=6$, asynchronous CPU scheduling,
and SparseAttn with a minimum
budget of 192 tokens. Sparse decoding and the full-attention AR reference
use the same rollout engine (Appendix~\ref{app:ssrl-implementation}). Each run
starts with 64 resident requests at context length 8192. We sweep configured
budgets $s_{\mathrm{cfg}}\in\{0.03,0.05,0.10,0.20,0.35,0.50\}$;
here K denotes 1024 tokens.

For each model, the first 192 distinct dense-AR continuations of DAPO
prompts that reach context 8192 without EOS form three disjoint bundles of
64 inputs, fixed across AR and all budgets. All runs use temperature one
and engine RNG seed 330. EOS is
disabled during timing, and the workload is conditional on survival to 8K.
Each configuration has 18 sparse runs and three AR references; the six
ratios within a bundle share one AR denominator. The primary configurations
are 1.7B/Graph160 and 8B/Graph640, with 8B/Graph160 as an additional control.

\paragraph{Timing and useful progress.}
Timing starts after at least 50 ready iterations, once mean committed
context reaches 8256, then covers at least 256 further committed tokens per
request on average. Sparse endpoints follow complete verification and commitment.
No requests enter or leave the active set during these windows, and no KV pages are offloaded. CUDA is drained
at both endpoints, with no added internal synchronization; the terminal
drain is included and the terminal TP barrier excluded. We use the larger
TP-rank time and require paired AR/sparse endpoint mean contexts to differ
by at most 32 tokens.

For committed output counts $Y$ and elapsed times $T$, each paired speedup is
\begin{equation}
 \eta_j=\frac{Y_{\mathrm{SS},j}/T_{\mathrm{SS},j}}
                  {Y_{\mathrm{AR},j}/T_{\mathrm{AR},j}}.
 \label{eq:why-ssrl-window-speedup}
\end{equation}
Progress counts accepted drafts plus one correction or bonus token per
completed request round, with $\tau_j=1+k\alpha_j$
(Appendix~\ref{app:why-ssrl-cost}). Effective $s_j$ is logical draft KV
reads divided by the corresponding full KV volume, including minimum-budget,
rounding, and appended-token effects. It is measured independently of
acceptance and time and does not measure physical HBM traffic.

\paragraph{Measured budget trade-off.}
Higher acceptance need not yield higher throughput
(Figure~\ref{fig:why-ssrl-budget-overlay}). Increasing the budget from 0.05 to
0.50 raises representative acceptance from 0.795 to 0.958 for 1.7B and
from 0.804 to 0.967 for 8B, while median speedup falls from
$1.533\times$ to $1.094\times$ and from $1.370\times$ to $1.058\times$.
Reducing the budget from 0.05 to 0.03 also lowers speedup, to $1.469\times$
and $1.307\times$. Both accepted progress and execution cost therefore matter.
The sampled 0.05--0.10 region performs well without resolving a unique
optimum.
Each plotted estimate uses the measured acceptance and effective budget
of the run with median speedup at that budget.

\begin{figure}[tbp]
 \centering
 \begin{subfigure}[t]{0.48\linewidth}
  \centering
  \includegraphics[width=\linewidth]{figs/why_ssrl_2/figs/subfigs/budget_tradeoff_1_7b.pdf}
  \caption{Qwen3-1.7B.}\label{fig:why-ssrl-budget-overlay-1-7b}
 \end{subfigure}\hfill
 \begin{subfigure}[t]{0.48\linewidth}
  \centering
  \includegraphics[width=\linewidth]{figs/why_ssrl_2/figs/subfigs/budget_tradeoff_8b.pdf}
  \caption{Qwen3-8B.}\label{fig:why-ssrl-budget-overlay-8b}
 \end{subfigure}
 \caption{Measured and estimated speedup across sparse budgets for
 (\subref{fig:why-ssrl-budget-overlay-1-7b}) Qwen3-1.7B and
 (\subref{fig:why-ssrl-budget-overlay-8b}) Qwen3-8B at $B=64$, initial $S=8$K, and $k=6$.
 Orange diamonds denote held-out medians; blue stars denote RL observations
 at an effective draft KV-read ratio of 5\%.}
 \label{fig:why-ssrl-budget-overlay}
\end{figure}

\subsection{Calibration of the component approximation}
\label{app:why-ssrl-calibration}

We normalize Eq.~\ref{eq:why-ssrl-mixed-latency} by the two-component AR
approximation, with attention fraction and projection scaling
\begin{equation}
 \rho=\frac{T_{\mathrm{Attn}}(M)}
 {T_{\mathrm{GEMM}}(B)+T_{\mathrm{Attn}}(M)},\qquad
 g_k=\frac{T_{\mathrm{GEMM}}\!\left(\frac{2k+1}{k+1}B\right)}
 {T_{\mathrm{GEMM}}(B)}.
 \label{eq:why-ssrl-calibration-anchors}
\end{equation}
The normalized round cost and ideal speedup are then
\begin{equation}
 D_0(s)=(k+1)g_k(1-\rho)+(1+ks)\rho,\qquad
 \eta_0=\frac{\tau}{D_0(s)}.
 \label{eq:why-ssrl-normalized-cost}
\end{equation}
We fix $\rho$ and $g_k$ from independent AR profiles before fitting.
The attention fraction uses $(B,S)=(64,8\mathrm{K})$ and excludes other
kernels and communication. For $g_k$, we interpolate projection costs at
$B=64$ and 128, measured at $S=4$K, to $B=118.86$. This is a proxy for
projection scaling in a mixed draft--verify pass at $S=8$K.

\paragraph{Calibration and held-out budgets.}
We fit the residual $\tau_j/\eta_j-D_0(s_j)$ on budgets 0.03, 0.10,
0.35, and 0.50 (12 equally weighted observations), holding out 0.05 and
0.20 (six observations). A linear residual replaces a constant only if
leave-one-calibration-budget-out cost RMSE improves by at least 20\% and
bundle-specific slopes agree in sign, with positive, nondecreasing cost on
$s\in[0.025,0.52]$. All three configurations select a constant $\delta$:
\begin{equation}
 \widehat\eta(\alpha,s)=\frac{1+k\alpha}{D_0(s)+\delta},\qquad
 \delta=\frac{1}{12}\sum_{j\in\mathcal C}
 \left[\frac{\tau_j}{\eta_j}-D_0(s_j)\right],
 \label{eq:why-ssrl-calibrated-speedup}
\end{equation}
where $\mathcal C$ is the calibration set and $k=6$. Held-out budgets and
RL timings enter neither fitting nor selection. The model takes measured
acceptance as input, with break-even condition
$\alpha>[D_0(s)+\delta-1]/k$.

\paragraph{Conditional speedup surfaces.}
Figure~\ref{fig:why-ssrl-surfaces} plots
Eq.~\ref{eq:why-ssrl-calibrated-speedup} over effective KV-read ratio $s$
and accepted-prefix fraction $\alpha$, using the primary configurations
in Table~\ref{tab:why-ssrl-fit}. At fixed $s$, higher acceptance increases
useful progress; at fixed acceptance, a larger budget raises attention cost.
The observations follow a workload-dependent $\alpha(s)$ trajectory, so
higher acceptance can accompany lower speedup. All measured points exceed
$1\times$; the break-even contour and low-acceptance region remain
conditional extrapolations beyond this trajectory.
The color scale saturates outside $0.5\times$--$2\times$.

\begin{figure}[tbp]
 \centering
 \newlength{\ssrlSurfacePanelWidth}
 \setlength{\ssrlSurfacePanelWidth}{0.43\linewidth}
 \begin{subfigure}[t]{\ssrlSurfacePanelWidth}
  \vspace{0pt}\centering
  \includegraphics[width=\linewidth]{figs/why_ssrl_2/figs/subfigs/surface_1_7b.pdf}
  \caption{Qwen3-1.7B.}\label{fig:why-ssrl-surface-1-7b}
 \end{subfigure}\hfill
 \begin{subfigure}[t]{\ssrlSurfacePanelWidth}
  \vspace{0pt}\centering
  \includegraphics[width=\linewidth]{figs/why_ssrl_2/figs/subfigs/surface_8b.pdf}
  \caption{Qwen3-8B.}\label{fig:why-ssrl-surface-8b}
 \end{subfigure}\hfill
 \begin{minipage}[t]{0.10\linewidth}
  \vspace{0pt}\centering
  \includegraphics[height=0.83\ssrlSurfacePanelWidth]{figs/why_ssrl_2/figs/subfigs/speedup_colorbar.pdf}
 \end{minipage}
 \par\medskip
 \includegraphics[width=0.90\linewidth]{figs/why_ssrl_2/figs/subfigs/surface_legend.pdf}
 \caption{Estimated speedup as a function of effective draft KV-read ratio and acceptance for
 (\subref{fig:why-ssrl-surface-1-7b}) Qwen3-1.7B and
 (\subref{fig:why-ssrl-surface-8b}) Qwen3-8B.
 Circles and diamonds denote calibration and held-out observations; the dark contour marks break-even.
 Blue stars denote RL observations at effective draft KV-read ratio $s=0.05$.}
 \label{fig:why-ssrl-surfaces}
\end{figure}

\begin{table}[t]
 \centering\small\setlength{\tabcolsep}{4pt}
 \input{figs/why_ssrl_2/tables/fit_summary}
 \caption{Component parameters, fitted residual, and errors on the six
 held-out observations. Ideal and Cal. denote predictions before and after
 calibration; MAPE and max. are mean and maximum absolute percentage errors.}
 \label{tab:why-ssrl-fit}
\end{table}

\paragraph{Execution costs beyond the approximation.}
Calibration reduces held-out MAPE from 84.61\% to 0.80\% for 1.7B and
from 63.03\% to 0.68\% for primary 8B. The residual combines execution
overhead with error in the projection-scaling proxy and AR normalizer.
Timed batches include synchronized drafting, verification, and no-forward
stalls that can expose unfinished GPU work. Sparse selection, communication,
and asynchronous waits further separate elapsed time from component costs.
The residual does not identify these contributions individually.

\subsection{Execution and workload sensitivity}
\label{app:why-ssrl-sensitivity}

\paragraph{Prediction versus measurement.}
Figure~\ref{fig:why-ssrl-prediction-parity} shows agreement between
calibrated and measured speedup along the observed budget trajectories.
It includes all 54 calibration and held-out observations across the three
configurations; Table~\ref{tab:why-ssrl-fit} isolates the held-out errors.

\paragraph{Execution configurations.}
Both 8B configurations show the same budget trade-off, with speedup
approaching $1\times$ at higher budgets
(Figure~\ref{fig:why-ssrl-execution-configurations}). KV capacity and
background CPU activity also differ, so this comparison does not isolate
CUDA Graph effects.

\begin{figure}[tbp]
 \centering
 \begin{subfigure}[t]{0.48\linewidth}
  \centering
  \includegraphics[width=\linewidth]{figs/why_ssrl_2/figs/subfigs/prediction_parity.pdf}
  \caption{Prediction versus measurement.}\label{fig:why-ssrl-prediction-parity}
 \end{subfigure}\hfill
 \begin{subfigure}[t]{0.48\linewidth}
  \centering
  \includegraphics[width=\linewidth]{figs/why_ssrl_2/figs/subfigs/execution_configurations_8b.pdf}
  \caption{8B execution configurations.}\label{fig:why-ssrl-execution-configurations}
 \end{subfigure}
 \caption{Execution sensitivity.
 (\subref{fig:why-ssrl-prediction-parity}) Predicted versus measured speedup across 54 profiling runs,
 with the diagonal denoting equality;
 (\subref{fig:why-ssrl-execution-configurations}) median speedup for the two Qwen3-8B execution configurations.}
 \label{fig:why-ssrl-execution}
\end{figure}

\paragraph{Changing batch or context.}
Table~\ref{tab:why-ssrl-states} varies batch or context at budget 0.05
using primary 1.7B and 8B/Graph160, with one input bundle per state,
excluded from fitting. EOS is disabled, so some 16K contexts extend beyond
an earlier EOS. Speedup varies with inference state; these diagnostics
do not validate transferring the $(64,8\mathrm{K})$ calibration unchanged.

\begin{table}[t]
 \centering\small
 \input{figs/why_ssrl_2/tables/state_diagnostics}
 \caption{Batch/context diagnostics at budget 0.05. Each row reports one
 paired throughput measurement without independent replication.}
 \label{tab:why-ssrl-states}
\end{table}

\subsection{Comparison with real RL rollouts}
\label{app:why-ssrl-rl}

We compare four paired 1.7B RL steps and three paired 8B steps with the
frozen local models. Each step generates eight responses per prompt for
256 prompts across four TP2 replicas, using full verification, CPU KV
offloading, and maximum concurrency 256 per replica. The AR baseline uses
vLLM, with prompt identities matched across methods; sampled outputs
and counts can differ.
The effective draft KV-read ratio for these RL observations is $s=0.05$.
% The authors confirmed the effective ratio on 2026-09-17; the previous
% 0.03/proxy wording was a stale placeholder.

\paragraph{RL markers in the surfaces and budget curves.}
Figures~\ref{fig:why-ssrl-budget-overlay} and
\ref{fig:why-ssrl-surfaces} show three steps per model. For 1.7B,
steps 72, 73, and 75 (a/b/c) are sampled uniformly without replacement from
steps 72--75 using seed 42; all four enter the aggregate comparison below.
For 8B, a/b/c show all available steps, 71/72/73. Stars use measured
acceptance and speedup at their effective ratio $s=0.05$.

\paragraph{Generation-throughput comparison.}
RL speedup compares aggregate output throughputs,
\begin{equation}
 \eta_{\mathrm{RL}}=
 \frac{\sum_t Y_{\mathrm{SS},t}/\sum_t T_{\mathrm{SS},t}}
      {\sum_t Y_{\mathrm{dense},t}/\sum_t T_{\mathrm{dense},t}}.
 \label{eq:why-ssrl-rl-speedup}
\end{equation}
Here $T$ is generation wall time, excluding RL optimization. These short
comparisons are separate from the main training runs. Aggregate acceptance
is total accepted drafts divided by total proposed drafts.

The measured aggregate speedups are $1.558\times$ for 1.7B and
$1.491\times$ for 8B, at acceptance 0.757 and 0.771. The primary local
models estimate $1.518\times$ and $1.352\times$, respectively
($-2.59\%$ and $-9.32\%$ relative to measurement). Applying the 8B control
calibration to the same three steps gives $1.321\times$ ($-11.41\%$).
% Numerical estimates retained as requested on 2026-09-17. This revision
% corrects the RL-marker ratio description only; no numerical refit is performed.
These runs support RL acceleration, but differences in workload, offloading,
AR baseline, and timing scope mean that local held-out errors do not quantify
RL prediction accuracy.
