# Supplementary material for: S$^3$R: Fast and Faithful RL Rollouts via Self-Sparse Speculative Decoding
Source: arXiv:2610.13202 source file (2026-11-03)
Supplement: Supplementary file 2 [file why_sparse_self_speculation.bak.tex]

% Paper-ready appendix section for the systems rationale of \modelname.
% Bibliography keys match the DBLP entries used in the main text.
% Expected packages: graphicx.

\section{Why Self-Sparse Speculative Decoding for RL Rollouts?}
\label{app:why-ssrl}

This appendix supports the latency discussion in
Section~\ref{sec:efficiency-runtime}. We decompose projection and
attention costs, derive a feasibility condition, and profile the components
across rollout workloads. Controlled budget sweeps in
Appendix~\ref{app:why-ssrl-budget} then measure accepted progress and
throughput together. Calibration, workload diagnostics, and separate RL
observations examine the scope of these local measurements.

\subsection{Latency decomposition for self-sparse speculative decoding}
\label{app:why-ssrl-cost}

We extend the serialized latency accounting in
Eq.~\ref{eq:efficiency-sd-accounting} by separating projection work from
historical KV reads at locally fixed active batch size $B$ and mean cached
context length $S$. For complete rounds, let $\alpha$ be the mean fraction
of the $k$ draft tokens accepted; then $\tau=1+k\alpha\in[1,k+1]$.

Let $T_{\mathrm{GEMM}}(B)$ cover QKVO, FFN, and LM-head work, and let
$T_{\mathrm{Attn}}(M)$ cover attention at aggregate KV volume
$M\propto B\cdot S$. The shared-weight drafter retains projection work but
reads a fraction $s\in(0,1]$ of the historical KV. We approximate
bandwidth-bound attention latency as linear in $M$. Verification processes
the $k$ drafts plus the preceding round's final token, whose dense KV is
not yet cached. Assuming $k+1\ll S$ and shared historical reads across
these $(k+1)B$ queries gives
\begin{equation}
\begin{aligned}
 T_p&=T_{\mathrm{GEMM}}(B)+T_{\mathrm{Attn}}(M),\\
 T_q&=T_{\mathrm{GEMM}}(B)+sT_{\mathrm{Attn}}(M),\\
 T_V&=T_{\mathrm{GEMM}}((k+1)B)+T_{\mathrm{Attn}}(M).
\end{aligned}
\label{eq:why-ssrl-sparse-stages}
\end{equation}
Projection latency need not scale linearly with $B$ because small batches
reuse weights. Larger batches can increase $T_V/T_p$, whereas longer
contexts at fixed $B$ push it toward one
\citep{sadhukhan2025magicdec,DBLP:journals/corr/abs-2606-18967}.

Shared weights also permit draft and verification queries in one forward.
With requests evenly staggered across $k$ draft stages and one verification
stage~\citep[Sections~3.2--3.3]{DBLP:journals/corr/abs-2512-01278},
each iteration has $kB/(k+1)$ single-query drafts and $B/(k+1)$
verifications of $k+1$ queries each. This yields $(2k+1)B/(k+1)$ queries
and $(ks+1)M/(k+1)$ effective KV reads per iteration. Each request
completes a round in $k+1$ iterations, so the mixed-stage cost per output
token is
\begin{equation}
 \frac{T_{\mathrm{mix}}}{\tau}
 =\frac{k+1}{\tau}\left[
 T_{\mathrm{GEMM}}\!\left(\frac{2k+1}{k+1}B\right)
 +T_{\mathrm{Attn}}\!\left(\frac{ks+1}{k+1}M\right)\right].
 \label{eq:why-ssrl-mixed-latency}
\end{equation}
By linearity, the attention term becomes $(ks+1)T_{\mathrm{Attn}}(M)/\tau$.

At full acceptance, $\tau=k+1$ maximizes output per round for fixed
$(B,S,s,k)$. Comparing Eq.~\ref{eq:why-ssrl-mixed-latency} with the AR
latency $T_p$ gives the ideal mixed-stage feasibility condition
\begin{equation}
 k(1-s)T_{\mathrm{Attn}}(M)
 >(k+1)\left[
 T_{\mathrm{GEMM}}\!\left(\frac{2k+1}{k+1}B\right)
 -T_{\mathrm{GEMM}}(B)\right].
 \label{eq:why-ssrl-full-acceptance}
\end{equation}
The left-hand side is the attention saving; the right-hand side is the
projection overhead from mixing draft and verification queries. If the
condition fails, no acceptance rate yields a speedup in this component
model. Observed acceleration also depends on actual acceptance and costs
beyond this approximation, examined in
Appendix~\ref{app:why-ssrl-calibration}.

\subsection{Component profiling setup}
\label{app:why-ssrl-setup}

We use $B$ for the active batch on one tensor-parallel (TP) rollout replica,
$S$ for the cached context length per request, and $N_{\mathrm{KV}}=B\cdot S$ for aggregate live
KV tokens in the fixed-length workloads. We use $1\mathrm{K}=1024$ tokens
for both context lengths and aggregate KV counts. Table~\ref{tab:why-ssrl-setup}
summarizes the common setting. Appendix~\ref{app:why-ssrl-e2} reports
acceptance thresholds in terms of $\alpha$, using $\tau=1+k\alpha$ from
Appendix~\ref{app:why-ssrl-cost}.

\begin{table}[t]
\centering
\small
\caption{Common setting for Appendices~\ref{app:why-ssrl-e1} and~\ref{app:why-ssrl-e2}.}
\label{tab:why-ssrl-setup}
\begin{tabular}{ll}
\hline
Item & Setting \\
\hline
Model & Qwen3-8B, DAPO step-60 checkpoint \\
Hardware & $2\times$NVIDIA H100 80GB HBM3 \\
Parallelism & one rollout-engine replica, TP${=}2$ \\
Precision & BF16 \\
Workload & equal-length synthetic prompts, fixed concurrency, ignore EOS \\
Sampling & temperature 0 (deterministic systems workload) \\
AR baseline & ordinary AR with full attention \\
Sparse draft & Pillar attention, ratio 0.05, minimum 192 tokens \\
Speculation & draft length $k=6$, exact full-model verification \\
\hline
\end{tabular}
\end{table}

We instrument scheduler iterations and model components with NVTX and collect
CUDA kernel traces using Nsight Systems. Attribution runs execute eagerly so
that the Python-level component ranges are visible. The profiles in
Appendix~\ref{app:why-ssrl-e1} use 50 ready-state warm-up iterations;
those in Appendix~\ref{app:why-ssrl-e2} use eight ready-state warm-up
iterations and one capture-settle iteration. Both record 20 measured
iterations. GPU component times are normalized per measured scheduler
iteration and per TP rank. For Appendix~\ref{app:why-ssrl-e1}, we assign
each classified kernel to its finest stable range and normalize component
shares by the sum of \emph{non-collective} GPU-kernel times. This excludes
topology-dependent TP collectives while retaining all memory traffic within
attention kernels. The attention profile in Appendix~\ref{app:why-ssrl-e2}
includes both draft and verification attention over all 20 scheduler states,
including two no-forward stall states. These profiles describe GPU work per
iteration; they do not normalize for differences in output length.

For the acceptance thresholds in Appendix~\ref{app:why-ssrl-e2}, $T_p$,
$T_q$, and $T_V$ are separately measured scheduler intervals, including CPU
time exposed around each GPU forward. Their sum $kT_q+T_V$ estimates sequential
stage costs and excludes no-forward stalls and cross-request phase mixing.
The synchronized workload does not isolate the scheduling mechanisms described in
Appendix~\ref{app:why-ssrl-cost}. Its thresholds are therefore
conditional on the measured stage costs; realized rollout speedup requires
matched end-to-end timing.

\subsection{Attention cost under rollout workloads}
\label{app:why-ssrl-e1}

We sweep $B\in\{1,4,16,32,64,128,256\}$ and
$S\in\{1,2,4,8,16,24,32\}\mathrm{K}$, subject to the measured KV-capacity
limit. This gives 35 feasible grid points.
We additionally profile $(B,S)=(8,2\mathrm{K})$ and $(2,4\mathrm{K})$, yielding
37 formal attribution traces in total.  The two added points complete the four
rollout-tail coordinates analyzed by EfficientRollout
~\citep{DBLP:journals/corr/abs-2606-18967}.

We group kernels into FFN, QKV and output projections (QKVO), attention, LM
head, and Other.  Other contains normalization, RoPE/KV append, elementwise,
embedding, sampling, and remaining scheduler GPU kernels.  Table~
\ref{tab:why-ssrl-e1-breakdown} first reproduces the small-$N_{\mathrm{KV}}$ rollout-tail
coordinates and then holds $B=16$ while increasing $S$.  Each component entry
is latency in milliseconds followed by its share of non-collective GPU-kernel
latency.

\begin{table*}[t]
\centering
\setlength{\tabcolsep}{5.5pt}
\caption{Decomposition of ordinary full-attention AR decoding.  Entries are
ms (percentage of the non-collective GPU-kernel total); TP collectives are
excluded from all columns and from the normalization.  The upper panel matches
the $(S,B)$ coordinates used in the rollout-tail analysis of
EfficientRollout~\citep{DBLP:journals/corr/abs-2606-18967}; the lower panel exposes the
long-context transition on our workload.}
\label{tab:why-ssrl-e1-breakdown}
\begin{tabular}{@{}rrrrrrrr@{}}
\hline
$N_{\mathrm{KV}}$ & $S$ & $B$ & Attention & FFN & QKVO & LM head & Others \\
\hline
8K   & 2K  & 4   & 0.96 (19.4\%)  & 2.18 (43.8\%) & 0.83 (16.6\%) & 0.21 (4.1\%) & 0.80 (16.1\%) \\
8K   & 4K  & 2   & 0.93 (18.8\%)  & 2.18 (44.2\%) & 0.82 (16.6\%) & 0.20 (4.2\%) & 0.80 (16.2\%) \\
8K   & 8K  & 1   & 0.98 (19.8\%)  & 2.17 (43.7\%) & 0.82 (16.5\%) & 0.20 (4.1\%) & 0.79 (16.0\%) \\
16K  & 2K  & 8   & 1.16 (22.4\%)  & 2.19 (42.1\%) & 0.83 (16.0\%) & 0.21 (4.0\%) & 0.81 (15.6\%) \\
\hline
64K  & 4K  & 16  & 2.34 (36.2\%)  & 2.24 (34.6\%) & 0.85 (13.2\%) & 0.21 (3.3\%) & 0.82 (12.7\%) \\
128K & 8K  & 16  & 3.85 (48.4\%)  & 2.23 (28.1\%) & 0.85 (10.7\%) & 0.21 (2.6\%) & 0.82 (10.3\%) \\
256K & 16K & 16  & 6.85 (62.4\%)  & 2.24 (20.4\%) & 0.85 (7.8\%)  & 0.21 (1.9\%) & 0.82 (7.5\%) \\
512K & 32K & 16  & 12.93 (75.8\%) & 2.24 (13.2\%) & 0.85 (5.0\%)  & 0.21 (1.2\%) & 0.82 (4.8\%) \\
512K & 16K & 32  & 12.98 (75.1\%) & 2.37 (13.7\%) & 0.87 (5.1\%)  & 0.21 (1.2\%) & 0.84 (4.9\%) \\
512K & 8K  & 64  & 13.11 (76.2\%) & 2.23 (13.0\%) & 0.76 (4.4\%)  & 0.21 (1.2\%) & 0.89 (5.2\%) \\
512K & 4K  & 128 & 13.07 (75.2\%) & 2.32 (13.4\%) & 0.80 (4.6\%)  & 0.22 (1.3\%) & 0.97 (5.6\%) \\
512K & 2K  & 256 & 13.44 (72.3\%) & 2.73 (14.7\%) & 0.99 (5.4\%)  & 0.24 (1.3\%) & 1.18 (6.3\%) \\
\hline
\end{tabular}
\end{table*}

At the four rollout-tail points, FFN, QKVO, and LM-head projections together
account for 62.1--65.0\% of non-collective kernel latency, while attention
accounts for 18.8--22.4\%.  This agrees qualitatively with the projection-bound
tail regime reported by EfficientRollout, despite differences in model,
hardware, TP degree, and measurement method.  The conclusion reverses as the
live KV volume grows: at $B=16$, attention rises from 2.34 ms at $S=4$K to
12.93 ms at $S=32$K, while FFN remains approximately 2.24 ms.

Figure~\ref{fig:why-ssrl-e1-ratio} shows the complete feasible grid as the
ratio of attention to FFN latency.  The ratio is below one in the small-$N_{\mathrm{KV}}$
tail, crosses one as aggregate live KV grows, and reaches 4.92--5.88 across the
feasible factorizations of $N_{\mathrm{KV}}=512$K.  Factoring the same $N_{\mathrm{KV}}$ differently also
gives similar ratios: 0.43--0.45 at $N_{\mathrm{KV}}=8$K, 0.97--1.12 at $N_{\mathrm{KV}}=64$K,
1.64--1.81 at $N_{\mathrm{KV}}=128$K, and 2.72--3.14 at $N_{\mathrm{KV}}=256$K.  Therefore neither $B$
nor $S$ alone describes the bottleneck.  For full-attention single-token
decoding in this range, their product $N_{\mathrm{KV}}=B\cdot S$ is the useful first-order
indicator of when KV-cache attention overtakes FFN.

\begin{figure}[t]
\centering
\includegraphics[width=0.68\linewidth]{figs/why_ssrl/e1_attention_ffn_heatmap.pdf}
\caption{Attention-to-FFN kernel latency ratio for full-attention AR decoding
across batch sizes and context lengths.
The black contour marks equal latency; hatched cells exceed the measured KV-capacity limit.}
\label{fig:why-ssrl-e1-ratio}
\end{figure}

\subsection{Drafting and verification costs}
\label{app:why-ssrl-e2}

We profile attention and draft--verify stage costs at eight feasible points
with $B\in\{16,32,64\}$ and $S\in\{4,8,16\}$K. Every reported value is the
median of three fresh profiling processes. These component measurements
complement the complete-window throughput measurements in
Appendix~\ref{app:why-ssrl-budget}.

\paragraph{Attention reduction.}
Table~\ref{tab:why-ssrl-e2-attention} compares attention GPU time in
full-attention AR and \modelname. The latter includes sparse drafting and
full-attention verification, averaged over the measured scheduler window.

\begin{table*}[t]
\centering
\small
\setlength{\tabcolsep}{6pt}
\caption{Attention profile.  Times are median NVTX GPU projections in ms per
measured scheduler iteration per TP rank over three processes.  \modelname includes
both sparse draft attention and full verification attention and is normalized
over all 20 scheduler states, including two no-forward stall states.  These are
component times, not per-output-token or end-to-end iteration times.}
\label{tab:why-ssrl-e2-attention}
\begin{tabular}{@{}rrrrrrr@{}}
\hline
$B$ & $S$ & $N_{\mathrm{KV}}$ & Full attention & \modelname attention & Saved & Reduction \\
\hline
16 & 4K  & 64K  & 2.31 & 1.42 & 0.88 & 38.3\% \\
16 & 8K  & 128K & 3.83 & 1.89 & 1.94 & 50.6\% \\
16 & 16K & 256K & 6.82 & 2.79 & 4.04 & 59.2\% \\
32 & 4K  & 128K & 3.80 & 1.96 & 1.84 & 48.5\% \\
32 & 8K  & 256K & 6.83 & 2.85 & 3.98 & 58.3\% \\
32 & 16K & 512K & 12.91 & 4.68 & 8.23 & 63.7\% \\
64 & 4K  & 256K & 6.91 & 2.90 & 4.02 & 58.1\% \\
64 & 8K  & 512K & 13.02 & 4.79 & 8.23 & 63.2\% \\
\hline
\end{tabular}
\end{table*}

The per-iteration attention saving rises from 0.88 ms at $N_{\mathrm{KV}}=64$K to
8.23 ms at $N_{\mathrm{KV}}=512$K, where the reduction reaches 63.2--63.7\%.
Similar savings across different $(B,S)$ factorizations of the same $N_{\mathrm{KV}}$
support aggregate live KV as an indicator of the available attention saving.

\paragraph{Draft and verification costs.}
For the measured stage costs, comparing $kT_q+T_V$ with the equal-output
AR cost $\tau T_p=(1+k\alpha)T_p$ gives the break-even acceptance
\begin{equation}
 \alpha_{\mathrm{BE}}^{\mathrm{stage}}
 =\frac{1}{k}\left(\frac{kT_q+T_V}{T_p}-1\right).
 \label{eq:why-ssrl-stage-threshold}
\end{equation}
Acceleration under this accounting requires
$\alpha>\alpha_{\mathrm{BE}}^{\mathrm{stage}}$.
Table~\ref{tab:why-ssrl-e2-stages} reports this threshold for $k=6$,
alongside the draft subtotal $6T_q$, verification cost $T_V$, and their
sum. The AR reference is $7T_p$, corresponding to full acceptance.

\begin{table*}[t]
\centering
\small
\setlength{\tabcolsep}{6pt}
\caption{Block-equivalent stage-time accounting for $k=6$.  AR max block is
$7T_p$, Draft subtotal is $6T_q$, and \modelname block is
$6T_q+T_V$.  Latencies (ms) are constructed
from medians over three process-level stage medians after aligning TP ranks and
selecting the critical rank.  Full AR and draft use CUDA Graphs; verification
is eager because its query batch $7B$ exceeds the capture bound. The
constructed block cost excludes no-forward stalls and cross-request phase
mixing (Appendix~\ref{app:why-ssrl-setup}).}
\label{tab:why-ssrl-e2-stages}
\begin{tabular}{@{}rrrrrrrr@{}}
\hline
$B$ & $S$ & $N_{\mathrm{KV}}$ & AR max block & Draft subtotal & Verify & \modelname block & $\alpha_{\mathrm{BE}}^{\mathrm{stage}}$ \\
\hline
16 & 4K  & 64K  & 54.42 & 40.06 & 28.06 & 68.12 & $>100\%$ \\
16 & 8K  & 128K & 65.55 & 39.15 & 27.97 & 67.12 & $>100\%$ \\
16 & 16K & 256K & 88.51 & 42.38 & 28.10 & 70.48 & 76.2\% \\
32 & 4K  & 128K & 66.70 & 40.89 & 29.03 & 69.92 & $>100\%$ \\
32 & 8K  & 256K & 88.12 & 43.01 & 26.86 & 69.87 & 75.8\% \\
32 & 16K & 512K & 133.18 & 43.73 & 28.56 & 72.29 & 46.7\% \\
64 & 4K  & 256K & 87.22 & 42.05 & 27.96 & 70.01 & 77.0\% \\
64 & 8K  & 512K & 129.85 & 42.51 & 26.68 & 69.19 & 45.5\% \\
\hline
\end{tabular}
\end{table*}

Under this accounting, even full acceptance cannot amortize the measured
stage costs at $N_{\mathrm{KV}}=64$K--128K. The threshold decreases to 75.8--77.0\% at
$N_{\mathrm{KV}}=256$K and 45.5--46.7\% at $N_{\mathrm{KV}}=512$K, while verification remains
substantial at 26.68--29.03 ms. Larger live KV volume thus creates more room
to amortize drafting and verification. These thresholds use separately
measured sequential stages; Eq.~\ref{eq:why-ssrl-full-acceptance} instead
assumes mixed-stage execution. The stage thresholds are not pooled with
the complete-window throughput measurements below.

\input{appendices/sparse_self_speculation_measurements}
